# Supplementary material for: Multimodal normative modeling in Alzheimers Disease with introspective variational autoencoders
Source: arXiv:2602.08077 source file (2026-02-08)
Supplement: Supplementary file 1 [file appendix.tex]

%%%%%%%%%%%%%%%%%%%%%%%%%%%%%%%%%%%%%%%%%%%%%%%%%%%%%%%%%%%%%%%%%%%%%%%%%%%%
% SUPPLEMENT / APPENDIX
%%%%%%%%%%%%%%%%%%%%%%%%%%%%%%%%%%%%%%%%%%%%%%%%%%%%%%%%%%%%%%%%%%%%%%%%%%%%
%\appendix

\section{Why the mmSIVAE game admits a consistent optimum (proof sketch)}
\label{app:nash}

This appendix provides an intuitive proof sketch for why the encoder--decoder game induced by the soft-introspective objective admits a consistent optimum in which (i) the learned model matches the reference data distribution and (ii) generated samples are discouraged from collapsing into the same posterior behavior as real samples.
Our goal is not to reproduce the full nonparametric analysis, but to state the key implication used in this work.

\paragraph{Setup.}
Let $p_{\mathrm{data}}(X)$ denote the reference (healthy) data distribution and $p_\theta(X)$ the model distribution induced by decoding $z\sim p(z)$ through $D_\theta$.
Let $q_\phi(z\mid X)$ denote the encoder and define the (scaled) ELBO terms for real and generated samples as in Eqs.~\eqref{eq:mmSIVAE_complete_encoder}--\eqref{eq:mmSIVAE_complete_decoder}.
The soft-introspective encoder loss contains an ``expELBO'' term that increases when generated samples have low ELBO (large reconstruction/KL terms), and the decoder loss encourages (a) good reconstructions of real data and (b) improved quality of generated samples, stabilized by $\gamma_r$ \cite{daniel2021soft}.

\paragraph{Claim (informal).}
Assuming the encoder and decoder families are sufficiently expressive, the game admits an optimum in which:
\begin{enumerate}
    \item the decoder matches the data distribution, $p_\theta(X)=p_{\mathrm{data}}(X)$, and
    \item the encoder yields consistent posteriors on real samples while assigning larger KL to generated samples early in training, preventing trivial solutions in which generated samples are immediately treated as real.
\end{enumerate}

\paragraph{Proof sketch.}
The argument follows the standard Soft-IntroVAE intuition \cite{daniel2021soft}:

\begin{enumerate}
    \item \textbf{Decoder consistency.}
    For fixed encoder, the decoder objective contains a reconstruction term on real samples and a KL-related term that penalizes mismatch between the aggregate posterior of real data and the prior.
    When optimized over a sufficiently expressive decoder, minimizing reconstruction error and matching latent usage encourages $p_\theta(X)$ to approach $p_{\mathrm{data}}(X)$.

    \item \textbf{Encoder discrimination via expELBO.}
    The encoder objective contains an expELBO term on generated samples (and reconstructions).
    Because the expELBO increases when the generated-sample ELBO is small, the encoder is incentivized to \emph{increase} $KL(D_\theta(z))$ (and/or reconstruction error for generated samples) relative to real samples.
    This creates a ``repulsion'' effect: generated samples are pushed away from the prior-matching behavior of real samples, preventing a degenerate fixed point where the encoder treats generated and real samples identically from the start.

    \item \textbf{Equilibrium behavior.}
    As the decoder improves, generated samples become more realistic and the decoder-side terms encourage better reconstructions and reduced KL for generated samples (modulated by $\gamma_r$).
    At equilibrium, when generated samples are indistinguishable from real samples in distribution ($p_\theta(X)=p_{\mathrm{data}}(X)$), the encoder no longer benefits from inflating $KL(D_\theta(z))$ because the generated-sample ELBO approaches the real-sample ELBO.
    Thus, the consistent optimum corresponds to matching the data distribution with stable inference.
\end{enumerate}

\paragraph{Takeaway for normative modeling.}
The key implication is that the introspective objective explicitly pressures the model toward a sharper fit of the reference distribution (via improved reconstructions and stabilized inference), which is beneficial when deviation scores rely on modeling the healthy cohort accurately.

%%%%%%%%%%%%%%%%%%%%%%%%%%%%%%%%%%%%%%%%%%%%%%%%%%%%%%%%%%%%%%%%%%%%%%%%%%%%
\section{MOPOE yields a valid ELBO (and subsumes PoE/MoE)}
\label{app:mopoe_elbo}

This appendix provides a compact derivation showing that MOPOE defines a valid ELBO and relates to PoE and MoE.

\paragraph{MOPOE posterior.}
Let $X=\{x_1,\ldots,x_N\}$ and let $\mathcal{P}(X)$ denote all non-empty modality subsets.
For any subset $S\in\mathcal{P}(X)$, define a PoE posterior
$q_{\mathrm{PoE}}(z\mid X_S)\propto p(z)\prod_{x_i\in X_S}q_{\phi_i}(z\mid x_i)$.
MOPOE is the uniform mixture over subsets:
\begin{equation}
q_{\mathrm{MOPOE}}(z\mid X)
=
\frac{1}{|\mathcal{P}(X)|}
\sum_{S\in\mathcal{P}(X)} q_{\mathrm{PoE}}(z\mid X_S).
\label{eq:supp_mopoe_def}
\end{equation}

\paragraph{ELBO validity.}
For any choice of approximate posterior $q(z\mid X)$, we have the standard identity:
\begin{equation}
\log p_\theta(X)
=
\mathcal{L}(X;q)
+
\mathrm{KL}\!\left(q(z\mid X)\,\|\,p_\theta(z\mid X)\right),
\label{eq:elbo_identity}
\end{equation}
where
\begin{equation}
\mathcal{L}(X;q)
=
\mathbb{E}_{q(z\mid X)}[\log p_\theta(X\mid z)]
-
\mathrm{KL}\!\left(q(z\mid X)\,\|\,p(z)\right).
\label{eq:generic_elbo}
\end{equation}
Because KL is non-negative, $\mathcal{L}(X;q)$ is a lower bound on $\log p_\theta(X)$.
Setting $q(z\mid X)=q_{\mathrm{MOPOE}}(z\mid X)$ yields a valid ELBO:
\begin{equation}
\mathcal{L}_{\mathrm{MOPOE}}(X)
=
\mathbb{E}_{q_{\mathrm{MOPOE}}(z\mid X)}
\Big[\sum_{i=1}^{N}\log p_\theta(x_i\mid z)\Big]
-
\mathrm{KL}\!\left(q_{\mathrm{MOPOE}}(z\mid X)\,\|\,p(z)\right).
\label{eq:mopoe_elbo}
\end{equation}

\paragraph{Relationship to PoE and MoE.}
MOPOE reduces to:
\begin{itemize}
    \item \textbf{PoE} when the mixture includes only the full set $S=X$, i.e., a single expert $q_{\mathrm{PoE}}(z\mid X)$ \cite{wu_multimodal_2018}.
    \item \textbf{MoE} when the mixture includes only singleton subsets $S=\{x_i\}$, producing $q(z\mid X)=\tfrac{1}{N}\sum_i q_{\phi_i}(z\mid x_i)$ \cite{shi2019variational}.
\end{itemize}
Thus MOPOE interpolates between the sharpness of PoE and the robustness of MoE by mixing PoE posteriors over subsets.

%%%%%%%%%%%%%%%%%%%%%%%%%%%%%%%%%%%%%%%%%%%%%%%%%%%%%%%%%%%%%%%%%%%%%%%%%%%%
